# Supplementary material for: Superconductivity-Enabled Conversion of Ferromagnetic Resonance into Standing Spin Waves
Source: arXiv:2604.27076 source file (2026-09-05)
Supplement: Supplementary file 1 [file SM_for_manuscript.tex]

\documentclass[%
  aps,
  prl,
  preprint,
  superscriptaddress,
  amsmath,amssymb,
  floatfix,
]{revtex4-2}

\usepackage[utf8]{inputenc}
\usepackage{graphicx}
\usepackage{bm}

\begin{document}

\begin{center}
\textbf{\large Supplemental Material for ``Superconductivity-Enabled Conversion of Ferromagnetic Resonance into Standing Spin Waves''}
\end{center}

% Prefix ``S'' to all counters
\setcounter{equation}{0}
\setcounter{figure}{0}
\setcounter{table}{0}
\renewcommand{\theequation}{S\arabic{equation}}
\renewcommand{\thefigure}{S\arabic{figure}}
\renewcommand{\bibnumfmt}[1]{[S#1]}
\renewcommand{\citenumfont}[1]{S#1}

\section{Additional experimental data}

\begin{figure}[t]
  \includegraphics[width=\linewidth]{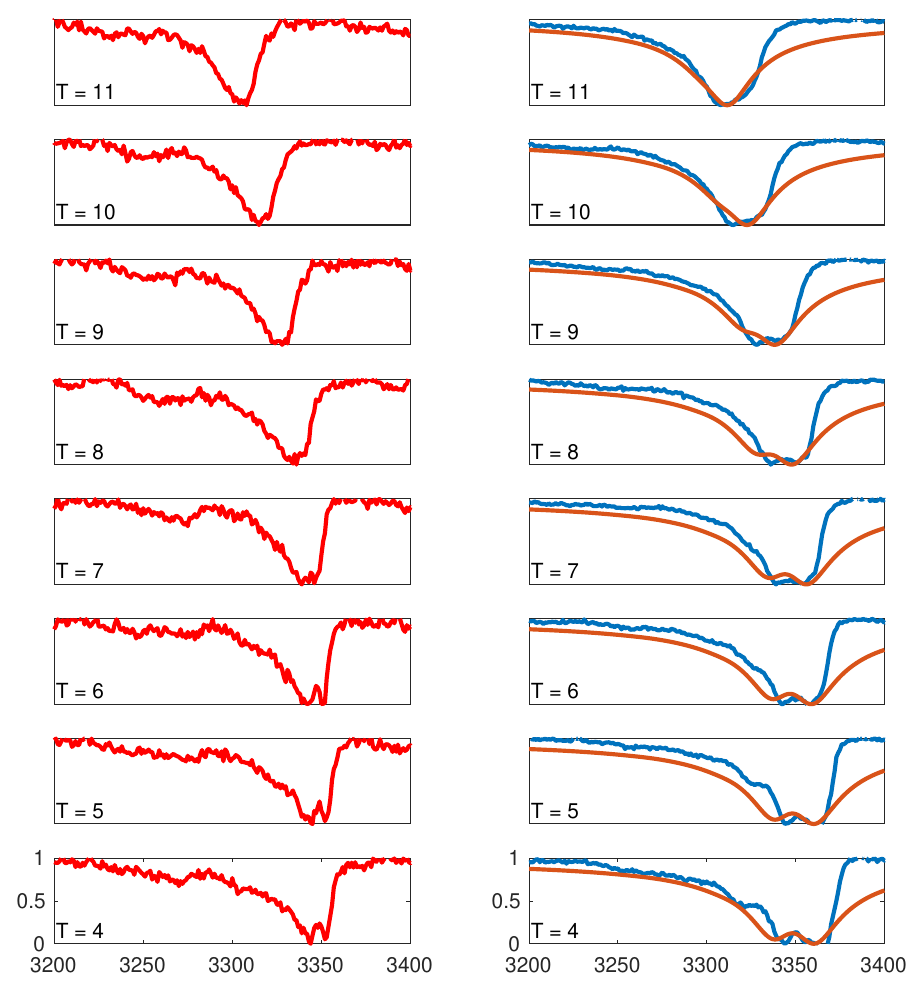}
  \caption{\label{fig:full_traces}
  Normalized microwave transmission $|S_{21}|$ versus out-of-plane field at $f=4$~GHz for temperatures $T=4$--11~K.
  Left column: uncapped Bi-GdIG film (experiment).
  Right column: Bi-GdIG/Nb bilayer (experiment, blue) together with the calculated lineshape (theory, orange).}
\end{figure}

Figure~\ref{fig:full_traces} shows the complete set of field-swept transmission spectra at $f=4$~GHz used for the comparison with theory in the main text.
The uncapped Bi-GdIG film exhibits the conventional FMR response \cite{lee2016ferromagnetic}.
A weak low-temperature splitting is attributed to a thin interfacial magnetic sublayer caused by substrate-element diffusion during growth \cite{lutsev2016low,lutsev2020spin}. It remains also when the structure is covered by the Nb film (right panel).
In the Bi-GdIG/Nb bilayer, an additional resonance feature (the ``right'' peak) develops only below the superconducting transition, while the ``left'' peak tracks the uncapped-film FMR position.

\section{Linearized Landau--Lifshitz--Gilbert equation}

We describe the magnetization dynamics in the ferrimagnetic layer by the Landau--Lifshitz--Gilbert (LLG) equation
\begin{equation}
\partial_t \mathbf{M}
= -\gamma\, \mathbf{M}\times \mathbf{H}_{\mathrm{eff}}
+ \frac{\alpha}{M_s}\,\mathbf{M}\times \partial_t\mathbf{M},
\label{eq:llg_full}
\end{equation}
where $M_s$ is the saturation magnetization, $\gamma$ is the gyromagnetic ratio, and $\alpha$ is the Gilbert damping.
For the out-of-plane configuration we use an effective field of the form
\begin{equation}
\mathbf{H}_{\mathrm{eff}}
= \mathbf{H}_{\mathrm{ext}}
+ \mathbf{H}_{\mathrm{SC}}(z)
-\frac{2A_{\mathrm{ex}}}{\mu_0 M_s^2}\,\partial_z^2\mathbf{M}
+ \mathbf{H}_{\mathrm{ani}}
- \hat{N}\mathbf{M}
+ \mathbf{h}_{\mathrm{AC}}(t),
\label{eq:Heff}
\end{equation}
where $A_{\mathrm{ex}}$ is the exchange stiffness, $\hat{N}$ is the demagnetizing tensor, $\mathbf{H}_{\mathrm{ani}}$ is the uniaxial-anisotropy contribution, and $\mathbf{h}_{\mathrm{AC}}(t)$ is the microwave drive.
The additional term $\mathbf{H}_{\mathrm{SC}}(z)$ accounts for the depth-dependent static field produced by Abrikosov vortices in the Nb film (electromagnetic proximity).

Linearizing about the equilibrium magnetization $\mathbf{M}_0 = M_s \mathbf{e}_z$ by writing $\mathbf{M}=\mathbf{M}_0+\mathbf{m}$ with $|\mathbf{m}|\ll M_s$ and keeping only transverse components of $\mathbf{m}$ yields the equation used in the main text,
\begin{equation}
\partial_t \mathbf{m}
= \gamma \bigl(H_0+H_{\mathrm{SC}}(z)\bigr)\,\mathbf{e}_z\times \mathbf{m}
+ \frac{2A_{\mathrm{ex}}\gamma}{\mu_0 M_s}\,\mathbf{e}_z\times \partial_z^2\mathbf{m}
+ \gamma M_s\,\mathbf{e}_z\times \mathbf{h}_{\mathrm{AC}},
\label{eq:llg_lin}
\end{equation}
where $H_0$ includes the external field and static internal contributions (anisotropy and demagnetizing field) appropriate for the saturated out-of-plane state.

\section{Interfacial spin torque and boundary condition}

To describe the spin-transfer torque at the FI/S interface we start from an interfacial $s$--$d$ exchange Hamiltonian,
\begin{equation}
\hat{H}_{\mathrm{int}}
= -J_{\mathrm{int}} \sum_{i\in \mathrm{int}}\hat{\mathbf{S}}_i\cdot \hat{\mathbf{s}}_i,
\label{eq:Hint}
\end{equation}
where $\hat{\mathbf{S}}_i$ and $\hat{\mathbf{s}}_i$ are the spin operators of a localized magnetic moment in the insulator and a conduction electron in the superconductor, respectively, and the sum runs over sites in a thin interfacial region.
Using the Ehrenfest theorem one obtains an interfacial torque density localized at $z=0$,
\begin{equation}
\mathbf{T}_{\mathrm{int}}
= -\gamma J\,\delta(z)\,\mathbf{M}\times \mathbf{s},
\label{eq:Tint}
\end{equation}
where $\mathbf{s}$ is the induced spin density in the superconducting film and $J$ is an effective interfacial exchange parameter that absorbs microscopic factors (interfacial thickness and lattice spacing).

Including Eq.~(\ref{eq:Tint}) in the LLG equation and integrating across a thin pillbox volume around the interface yields the boundary condition
\begin{equation}
\frac{2A_{\mathrm{ex}}}{\mu_0 M_s^2}\,\mathbf{M}\times \partial_z\mathbf{M}\Big|_{z=0}
- J\,\mathbf{M}\times \mathbf{s}\Big|_{z=0}
=0,
\label{eq:bc_full}
\end{equation}
which is a Robin-type condition analogous to interfacial pinning conditions in spin-wave theory \cite{rado1959spin,gurevich1996magnetization}.

Linearizing Eq.~(\ref{eq:bc_full}) with $\mathbf{M}=\mathbf{M}_0+\mathbf{m}$ and $\mathbf{s}=\mathbf{s}_0+\mathbf{s}$ gives
\begin{equation}
\mathbf{e}_z\times \partial_z \mathbf{m}\Big|_{z=0}
=
\zeta\Bigl(\mathbf{S}_0\times \mathbf{m} - \mathbf{M}_0\times \mathbf{s}\Bigr)\Big|_{z=0},
\label{eq:bc_lin_vec}
\end{equation}
where $\zeta=\mu_0 M_s^2 J /(2A_{\mathrm{ex}})$ and $\mathbf{S}_0$ is the stationary interfacial magnetization induced in the superconductor by $\mathbf{M}_0$.
In linear response we write
\begin{equation}
\mathbf{S}_0=\chi_0\,\mathbf{M}_0,
\qquad
\mathbf{s}=\chi(\Omega)\,\mathbf{m},
\label{eq:sus_defs}
\end{equation}
with the static and dynamic interfacial spin susceptibilities $\chi_0$ and $\chi(\Omega)$.
Substituting Eq.~(\ref{eq:sus_defs}) into Eq.~(\ref{eq:bc_lin_vec}) yields the compact form used in the main text,
\begin{equation}
\mathbf{e}_z \times \partial_z \mathbf{m}\big|_{z=0}
= \zeta\bigl[\chi(\Omega)-\chi_0\bigr]\;\mathbf{e}_z\times \mathbf{m}\big|_{z=0}.
\label{eq:bc_main}
\end{equation}

%\section{Vortex-induced depth-dependent field}

\section{Calculation of the magnetic susceptibility}

Equations~(\ref{eq:llg_lin}) and (\ref{eq:bc_main}), together with the free boundary condition at the FI/substrate interface ($\partial_z\mathbf{m}|_{z=d_{\mathrm{FI}}}=0$), define a linear boundary-value problem for $\mathbf{m}(z)$ at given frequency and field.
We discretize the film along $z$ and solve the resulting linear system to obtain the spatial profile $\mathbf{m}(z)$ and the spatially averaged response $\langle \mathbf{m}\rangle$.
The transverse susceptibility $\chi_{xy}$ shown in the main text is extracted from $\langle \mathbf{m}\rangle$ in the standard way.

Magnetic susceptibility of the insulator requires the solution of the  LLG equation.To calculate magnetic susceptibility, lets transform equation (S3) in unitless form, changing variables:
\begin{align}
    t \rightarrow \frac{t}{\gamma M_s} , z  \rightarrow z\sqrt{\frac{2 A_{ex}}{\mu_0 M_{s}^{2}}} \\
    M_0 \rightarrow {m_0}M_s, {\bf m} \rightarrow {\bf m}{M_s}, 
    {\bf H} \rightarrow {\bf h} M_s
\end{align}
After substitutions (S9) equation takes the form:
\begin{equation}
    \partial_t {\bf m} = 
    \left( h\left( z\right)
    - 1 \right)\mathcal{Q} {\bf m}
    - \mathcal{Q}\partial_{z}^{2}{\bf m}
    -  m_0 \mathcal{Q} {\bf h}_{AC},
\end{equation}
where $h\left( z\right)$ is the phenominilogical magnetic field describes the distortion induced by Abrikosov vortex lattice.

In the out-of-plane mixed state, vortex currents in the Nb film produce a static field correction that decays away from the interface on a characteristic ``healing'' length scale set by superconducting parameters \cite{tinkham2004introduction}.
To model this effect we use a simple piecewise-linear profile
\begin{subequations}
\begin{eqnarray}
h(z) = \left(  k_{s}z  - \left(H_{0} - M_{sc}\right) \right)/M_s,
0 \leq  z  <  L_{H}
\label{appa}
\\
h(z) = H_{0}/M_{s}, \label{appb}
 z >  L_{H}
\end{eqnarray}
\end{subequations}
where $h\left( z\right)$ parameterizes the interfacial field reduction due to screening and $L_H$ is an effective penetration depth of the vortex stray field into the garnet.

The matrix $\mathcal{Q}$ is obtained from the linearized LLG equation:
\begin{equation}
    \mathcal{Q} =  \left(\mathcal{I} -  \frac{\alpha M_0 }{M_{s}}\mathcal{E}\right)^{-1}
    \mathcal{E} = 
    \begin{bmatrix}
    -\frac{\alpha \frac{M_0}{M_s}}{\alpha^{2}\frac{M_0^2 }{M_{s}^2}+1} & -\frac{1}{\alpha^{2}\frac{M_0^2 }{M_{s}^2}+1} & 0\\
    \frac{1}{\alpha^{2}\frac{M_0^2 }{M_{s}^2}+1} &  -\frac{\alpha \frac{M_0}{M_s}}{\alpha^{2}\frac{M_0^2 }{M_{s}^2}+1} & 0\\
    0 &  0 & 0
    \end{bmatrix}
\end{equation}
Here $\mathcal{E}$ is the second Pauli matrix mutiplied by $i$ and extended to 3 by 3.
The magnetic vortex field varies at the scale of 10-20 nm  \cite{tinkham2004introduction} and creates the noticeable asymmetry of the PSSWs spectrum and thus, increase the excitation efficiency by the uniform alternating field. 
All entities in equation (S13) are now dimensionless. Unfortunately, the eigenvalues of equation (S13) cannot be fully resolved analytically even for the linear distribution of the stationary magnetic field $h(z)$. But the eigen-frequencies and eigenfunctions can be calculated numerically using finite-differences method for the wide range of the external magnetic fields and arbitrary distributions of vortex-lattice fields. The  finite-difference grid along the $z$ - direction is defined:
\begin{align}
       \mathcal{Z}_{h} = \left\{ z_j \in \mathbb{R} \;\middle|\; z_j = z_{\min} + j h,\ j = 0, 1, \dots, N \right\},
\end{align}
where $ z_{\min} = 0$ and $ z_{\max} = L_{z}/l_{ex}$ are the physical boundaries of the domain, $ h = \dfrac{z_{\max} - z_{\min}}{N}$ is the uniform mesh spacing, $N$ is the number of intervals, $N + 1$ is the total number of mesh points. The equation (S13) projected onto grid (S15) takes the form:
\begin{equation}
    \partial_t {\bf m}_{j} = 
    \left( h_{j}
    - 1 \right)\mathcal{Q} {\bf m}_{j}
    - \sum_{k = 0}^{N + 1}\mathcal{D}_{jk}{\bf m}_{k}
    -  m_0 \mathcal{Q} {\bf h}_{AC}.
\end{equation}
where $h_{j} = h\left( z_{j}\right)$ is the field in the $j^{th}$ grid point, $\mathcal{D}_{jk}$ is the 3x3 matrix of the second order derivative operator on the mesh (S15). The system of differential equations (S19) can be formally diagonalized and integrated if eigenvalues and eigen vectors of the linear operator $\mathcal{L}$ are known:
\begin{equation}
    \partial_t {\bf m} = \mathcal{L}{\bf m}
\end{equation}
Where ${\bf m}$ is the $3N$x$1$ vector containing $N$ $3$x1 vectors for every point in the $\mathcal{Z}_{h}$ finite-difference grid. The overall linear operator $\mathcal{L}$ for the ode system (S17) has dimensions $3N$x$3N$ correspondingly. Vector ${\bf m}$ and operator $\mathcal{L}$ exist in the linear space combined from the grid subspace $\mathcal{Z}_{h}$ and projections subspace $\mathcal{P}_{3}$: $\mathcal{Z}_{h} \otimes \mathcal{P}_{3}$. Using that fact,  $\mathcal{L}$ can be written using the Kronecker product:
\begin{equation}
    \mathcal{L} = \left( \operatorname{diag}(\mathbf{h}) - \mathcal{I} \right)
    \otimes \mathcal{Q} - \mathcal{D}_{z}\otimes\mathcal{Q}
\end{equation}
where $\operatorname{diag}(\mathbf{h})$ is the $N$x$N$ matrix containing values of stationary magnetic field at the very point of the mesh,  $\mathcal{D}_{z}$ is the  is the $N$x$N$ tridiagonal matrix of the second order derivative operator on the finite-difference grid with proper boundary conditions (S9). Modes and frequencies of hybrid structure  can be numerically calculated from the following eigenproblem:
\begin{equation}
    \mathcal{L} {\bf V}_n = \lambda_n {\bf V}_n
\end{equation}
Where ${\bf V}_n$ are eigenvectors and $\lambda_n$  eigenvalues of the $\mathcal{L}$  finite difference operator. Eigen vectors are orthonormal and conserve the same subspace structure:
\begin{equation}
    {\bf V}_{n} =  \left[\begin{array}{c}
    {\bf V}_{n}^{(1)}\\
    {\bf V}_{n}^{(2)} \\
    {\bf V}_{n}^{(3)} \\
    \vdots \\
    {\bf V}_{n}^{(N)}
    \end{array} \right],
    \mathcal{V} = \begin{bmatrix}
    {\bf V}_{1}^{(1)} & {\bf V}_{2}^{(1)}& \dots &{\bf V}_{M}^{(1)} \\
    {\bf V}_{1}^{(2)} & {\bf V}_{2}^{(2)}& \dots &{\bf V}_{M}^{(2)} \\
    \vdots & \vdots & \ddots & \vdots \\
    {\bf V}_{1}^{(N)} & {\bf V}_{N}^{(2)}& \dots &{\bf V}_{M}^{(N)}
     \end{bmatrix}, 
\end{equation}
where $M$ - is the number of eigen-modes calculated from the problem (S19). The matrix $\mathcal{L}$ is a large sparse matrix (about $10^6$ elements and more) however the number of nonzero elements is about $10^{3} - 10^{4}$. The number of eigen-modes calculated from problem (S19) is usually $M \approx 5-15$ i.e $M \ll N$. So instead of the inverse matrix $\mathcal{V}^{-1}$ it is convenient to define $\mathcal{U} = \left( \mathcal{V}^{T} \mathcal{V}\right)^{-1}$. It gives: $\mathcal{U}\mathcal{V} = \mathcal{I}$. The structure of matrix $\mathcal{U}$ is very similar to $\mathcal{V}$:
\begin{equation}
    \mathcal{U} = \begin{bmatrix}
    {\bf U}_{1}^{(1)} & {\bf U}_{1}^{(2)}& \dots &{\bf U}_{1}^{(N)} \\
    {\bf U}_{2}^{(1)} & {\bf U}_{2}^{(2)}& \dots &{\bf U}_{2}^{(N)} \\
    \vdots & \vdots & \ddots & \vdots \\
    {\bf U}_{M}^{(1)} & {\bf U}_{M}^{(2)}& \dots &{\bf U}_{M}^{(N)}
     \end{bmatrix} ,
\end{equation}
where vectors $ {\bf U}_{m}^{(j)}$ satisfy the following condition:
\begin{equation}
    \mathcal{U}\mathcal{V} = \mathcal{I} \rightarrow
    \sum_{j = 1}^{N} {\bf U}_{m}^{(j)}{\bf V}_{n}^{(j)} = \delta_{mn},
\end{equation}
where $\delta_{mn}$ is the Kronecker's delta symbol. Matrices $\mathcal{V}$ and $\mathcal{U}$ diagonalize operator $\mathcal{L}$:
\begin{equation}
    \mathcal{U}\mathcal{L}\mathcal{V}= 
    \operatorname{diag}\left( {\bf \lambda}\right) \rightarrow
    \sum_{j = 1}^{N}\sum_{k = 1}^{N} 
    {\bf U}_{m}^{(j)}\mathcal{L}_{ik}{\bf V}_{n}^{(k)} = \lambda_{n}\delta_{mn},
\end{equation}
where $\mathcal{L}_{ik}$ is 3x3 sub-block of $\mathcal{L}$ and $\lambda_{mn} = $. 
\begin{equation}
    \partial_t{\bf m }_{j} = 
    \sum_{k = 1}^{N}\mathcal{L}_{jk}
    {\bf m }_{k} 
    -  m_0 \mathcal{Q} {\bf h}_{AC}.,
\end{equation}
Linear ode system (S24) can be solved using (S22) and (S23) eigenvector matrices. The magnetization vector for the j-th  cell ${\bf m }_{J}$, can be represented: 
\begin{equation}
    {\bf m}_{j}\left( t \right) = \sum_{n = 1}^{M}
    {\bf V}_{n}^{(j)} c_{n}\left( t \right)
\end{equation}
Substituting (S25) into (S24) and multiplying the resulting matrix system  on $\mathcal{U}$ from the left side, taking into account (S22) we get diagonalized system:
\begin{equation}
\partial_tc_n = 
\lambda_{n}
    c_{n}  -  
    m_0 
    \sum_{j = 1}^{N}{\bf U}_{n}^{(j)}
    \mathcal{Q}
    {\bf h}_{AC}.,
\end{equation}
Let ${\bf h}_{AC} = {\bf h}e^{-i\Omega t}$, the ode system can now be formally solved and transformed back to solutions for magnetization vectors at every coordinate. After the magnetization averaging we get the following:
\begin{equation}
    \langle {\bf m}\rangle  
    = - i \sum_{n = 1}^{M}
    \frac{{\bf v}_n \otimes {\bf w}_n }{\omega_n - \Omega  + i\delta_n}{\bf h}
    e^{-i\Omega t}
\end{equation}
where ${\bf v}_{n}$,${\bf w}_{n}$ and average magnetization equal:
\begin{equation}
    {\bf v}_{n} =
    \frac{1}{N}
    \sum_{j = 1}^{N}
    {\bf V}_{n}^{(j)},
\end{equation}
\begin{equation}
    {\bf w}_{n} = 
    m_{0}
    \sum_{i = 1}^{N}
    {\bf U}_{n}^{(j)}\mathcal{Q},
\end{equation}
\begin{equation}
    \langle {\bf m}\rangle = 
    \frac{1}{N}\sum_{j = 1}^{N}
    {\bf m}_{j}
\end{equation}
Finally, the magnetic susceptibility equals:
\begin{equation}
    \chi \left( \Omega \right) 
    = - i \sum_{n = 1}^{M}
    \frac{{\bf v}_n \otimes {\bf w}_n }{\omega_n - \Omega  + i\delta_n}
\end{equation}
Equation (S31) was used to evaluate the response in the main text. Parameter values were used: $A_{ex}\approx 0.01 - 0.2$ pJ/m, $\alpha \approx 0.01 - 0.05$.

\section{Saturation magnetization calculation}

\begin{figure}[h]
  \includegraphics[scale=0.8]{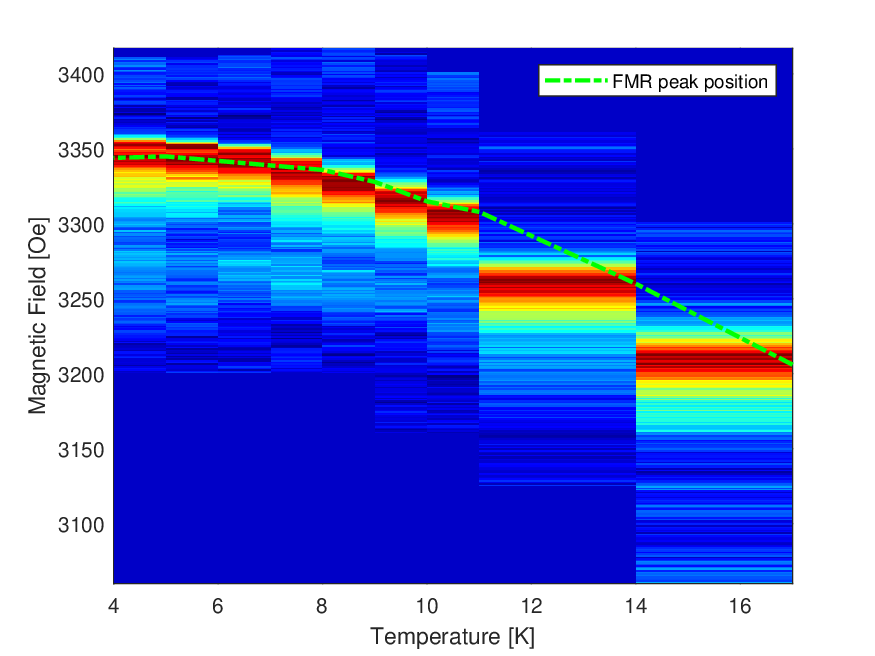}
  \caption{\label{fig:full_traces}
  Normalized microwave transmission $|S_{21}|$ and FMR peak position versus out-of-plane field and temperature at $f=4$~GHz for uncapped Bi-GdIG film}
\end{figure}

Saturation magnetization in our model is a temperature dependent quantity. It strongly depends on the temperature because of Gadolinium sublattice in the substituted garnet dramatically increases with the lowering of the temperature, the same effect takes on in the GGG substrate. Moreover, the FMR peak asymmetry which demonstrated in FIG 2 of the main text can be explained with the non-uniform magnetization, created by the strongly paramagnetic GGG substrate at the lower temperatures. The change of the effective saturation magnetization is calculated by the fitting FMR condition from the measured Bi-GdIG/GGG structure (FIG S2).

\end{document}
